# Supplementary material for: Radiation Brightening from Virus-like Particles
Source: arXiv:1907.00065 ancillary file (2019-07-02)
Supplement: Supplementary file 1 [file IrinaBMVCollectiveFluo_ACS_Nano_Supporting_information_Revision3-3.pdf]

# Supporting information for

# Radiation Brightening from Virus-like Particles under Pulsed Illumination

Irina B. Tsvetkova[a], Arathi Anil Sushma[a], Joseph C.-Y. Wang[b], William L. Schaich[c], and Bogdan G. Dragnea[a]*

[a]Chemistry Department, Indiana University Bloomington, IN, 47405, USA

[b]Department of Molecular and Cellular Biochemistry, Indiana University Bloomington, IN, 47405, USA

[c]Physics Department, Indiana University Bloomington, IN, 47405, USA

*Correspondence and requests for materials should be addressed to B.D. (email: dragnea@indiana.edu)

**Virus Modification and Characterization**

Virions of the Brome mosaic virus (BMV), with T = 3 icosahedral symmetry provided the symmetric template for bio-conjugation[1]. The 28 nm-diameter BMV capsid is composed of 180 identical copies of a single coat protein. BMV can be disassembled into protein dimers and RNA genome and reassembled[2]. Conditions for obtaining empty virus-like particles [3] or hybrid nanoparticles containing synthetic cores[4-6] have been extensively explored.

The chemical surface modification of BMV capsid has been studied [7]. wtBMV has 12 lysines per coat protein among which residues K64, K83, K105, K111, and K165 (Fig. 1A, S1) are surface-exposed and have been shown to efficiently undergo chemical modification by thioimidate reagents [8]. These reactive lysines provide, in principle, for 900 possible labeling sites on the virus surface, for further modification. We analyzed the likelihood of dye locations and nearest-neighbor distances on the surface of BMV by measuring distances between lysines residues in the full virus molecular model using the Chimera software. The average nearest distance between reactive surface exposed lysines is about 2 nm (Fig. SI1).

Lysines are commonly addressed through reaction with active esters (e.g, succinimidyl, sulfosuccinimidyl, or tetrafluorophenyl esters) [9] (Fig. 1B). Here, we used Oregon Green™ 488 carboxylic acid succinimidyl ester (OG). The average number of chromophores conjugated to the virus (N) was varied by changing the molar ratio of chromophores to the virus in the reaction media. The labeling reaction was done in two buffer conditions to obtain better control over N. Fig. SI2 shows the dependence of <N> on the dye input concentration at the reaction onset.

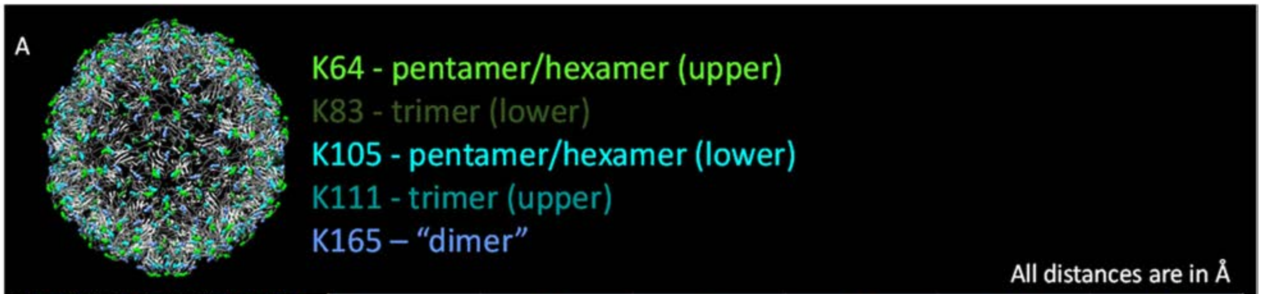


B

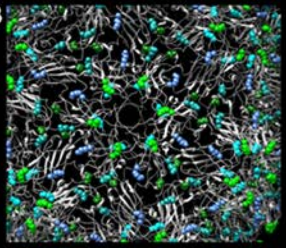

| hexamer | 64 | 83 | 105 | 111 | 165 |
|---|---|---|---|---|---|
| 64 | 18-20 | 34-39 | 11-18 | 27-28 | 23-25 |
| 83 | 34-39 | 13-18 | 27-29 | 11-15 | 21-24 |
| 105 | 11-18 | 27-29 | 18-19 | 24-25 | 20-21 |
| 111 | 27-28 | 11-15 | 24-25 | 14-19 | 22-24 |
| 165 | 23-25 | 21-24 | 20-21 | 22-24 | 16 |

C

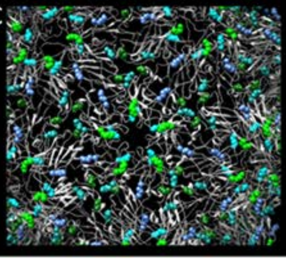

| pentamer | 64 | 83 | 105 | 111 | 165 |
|---|---|---|---|---|---|
| 64 | 17-28 | 32-38 | 9-17 | 27-39 | 24-26 |
| 83 | 32-38 | 13-18 | 28-35 | 11-15 | 21-24 |
| 105 | 9-17 | 28-35 | 13-21 | 27-34 | 24-27 |
| 111 | 27-39 | 11-15 | 27-34 | 14-19 | 22-24 |
| 165 | 24 -26 | 21-24 | 24-27 | 22-24 | 16 |

Figure SI1. Analysis of distances between possible labelling sites. A) Full virus model and color description, B) hexamer view and table with distances for hexameric subunit, C) same as B but for pentameric subunit. Note: From structure analysis K165, K64, K11 are likely to be labelled and K83 and K105 are less likely.

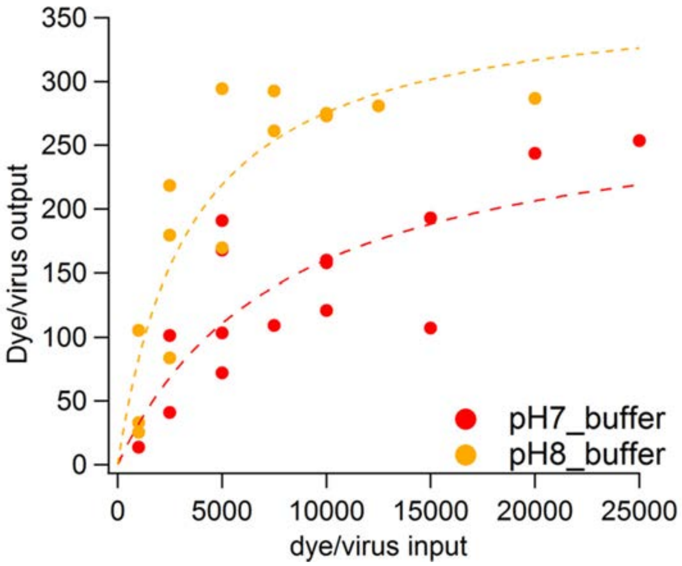


Figure SI2. Bioconjugation reaction output vs dye input in reaction mixture for two buffer conditions (dashed lines are binding isotherm fitting).

The efficiency of labeling in BMV-chromophore conjugates was determined by UV-Visible absorption spectroscopy and supported by Matrix Assisted Laser Desorption/Ionization-Time of Flight Spectrometry (MALDI-TOF). The average number of chromophores per particle was calculated from extinction data using the Beer-Lambert law. The molar extinction coefficient for Oregon green at 496 nm in buffer at pH 8 is $\varepsilon = 70{,}000 cm^{-1}M^{-1}$. BMV is most stable in buffers with pH 4-5. Therefore concentration measurements were done in these conditions. As a consequence of the pH change, the extinction coefficient had to be adjusted. In order to do account for the change in the extinction coefficient, the free dye absorbance spectrum was measured for a pH range from 4 to 8 at varied concentrations from 0.05 uM to 0.5 uM. Thus, we obtained an ε at pH 4.6 of $33641 cm^{-1}M^{-1}$.

MALDI-TOF (Fig. SI3) was used to provide molecular weight information of labeled proteins. For BMV labeled through lysine modification, there are two peaks present below 200 dyes/virus, which correspond to unlabeled protein and proteins with one dye. For samples with a dye/virus ratio of above 200, a third peak appeared which corresponds to two dyes per coat protein. Also, the height of unlabeled protein peak decreased significantly. By fitting the peaks, we can estimate the degree of labeling from MALDI experiments. The table in Figure SI3 provides the comparison between the labeling load calculated from UV-Vis spectra and from MALDI-TOF spectra. Although there is a difference in absolute numbers between two methods, the trend is the same. It is likely that MALDI-TOF underestimates the degree of labeling due to the particle stability against laser-induced fragmentation being dependent on labeling.

Particle morphology was imaged by negative stained TEM and Cryo-EM images and dye-conjugated BMV is indistinguishable from wtBMV (Fig. SI4). The inset in Fig SI4A shows the

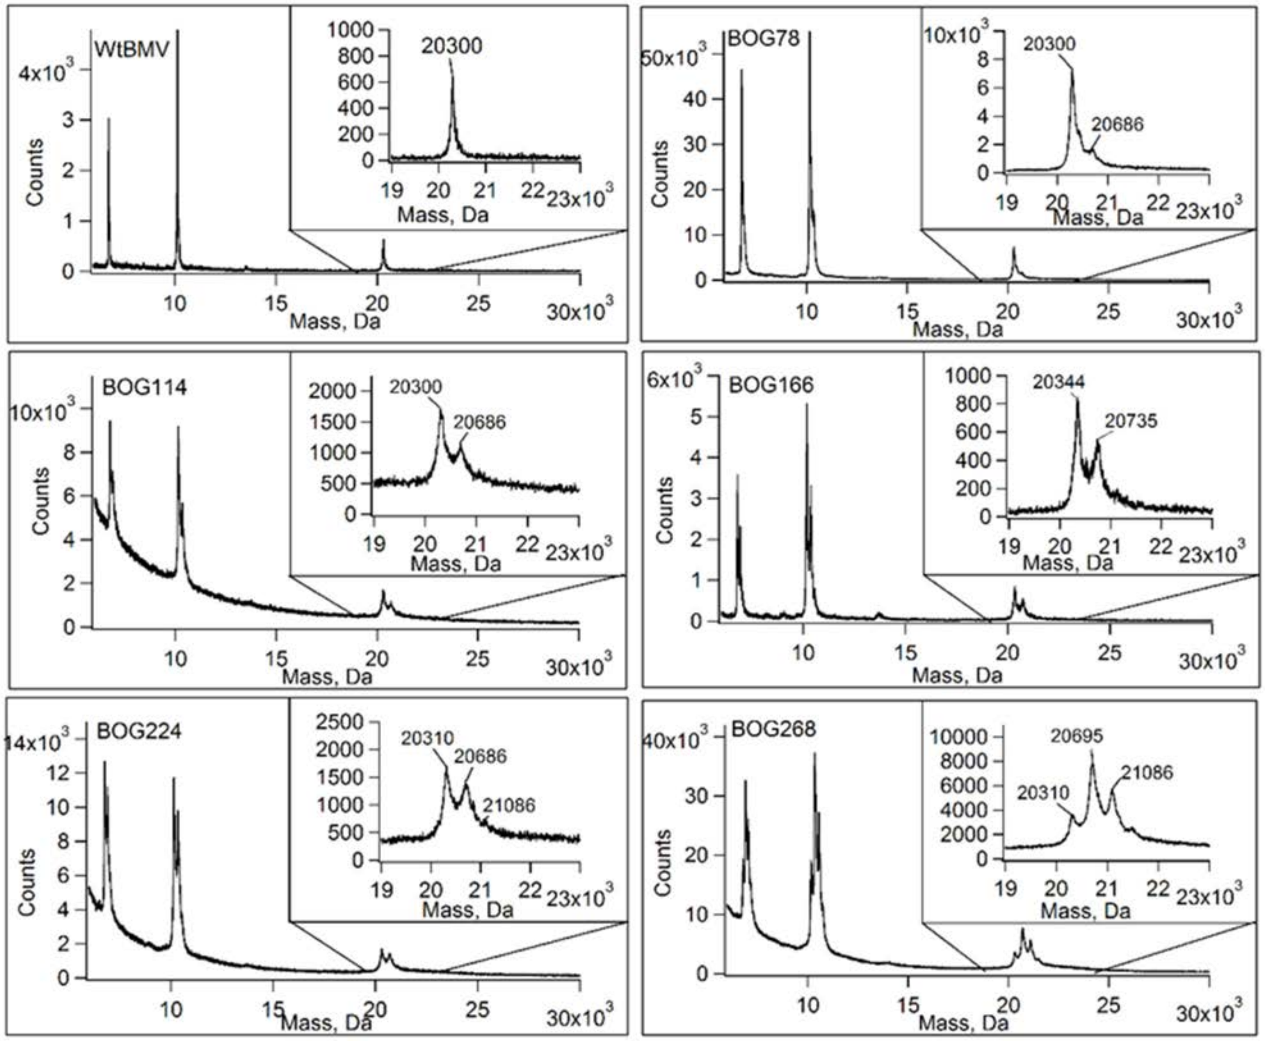


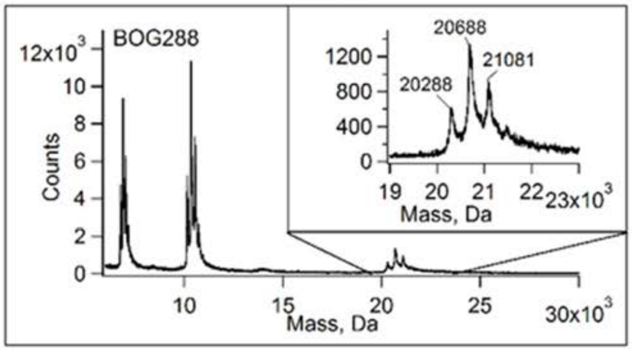


| Uv-Vis | MALDI-TOF |
|---|---|
| 78 | 30 |
| 114 | 65 |
| 166 | 75 |
| 224 | 125 |
| 268 | 223 |
| 288 | 250 |

Figure SI3. MALDI-TOF spectra for wtBMV and bioconjugated samples with different N and table with comparison of dye loading calculated from UV-Vis and MALDI spectra.

rotationally averaged particle image with two structural layers: the outer capsid layer and the inner RNA layer. No observable disruption on the labeled capsid surface can be detected (Fig SI4B). A total of 12522 particles from 141 micrographs were used to compute the final 3D reconstruction to 7Å resolution (estimated by Fourier shell correlation at 0.143). At the 3D level, the labeled BMV capsid also exhibits an overall architecture of T=3 surface lattice that is comparable to the native virus (Fig SI4C). There are 12 pentameric capsomer protrusions

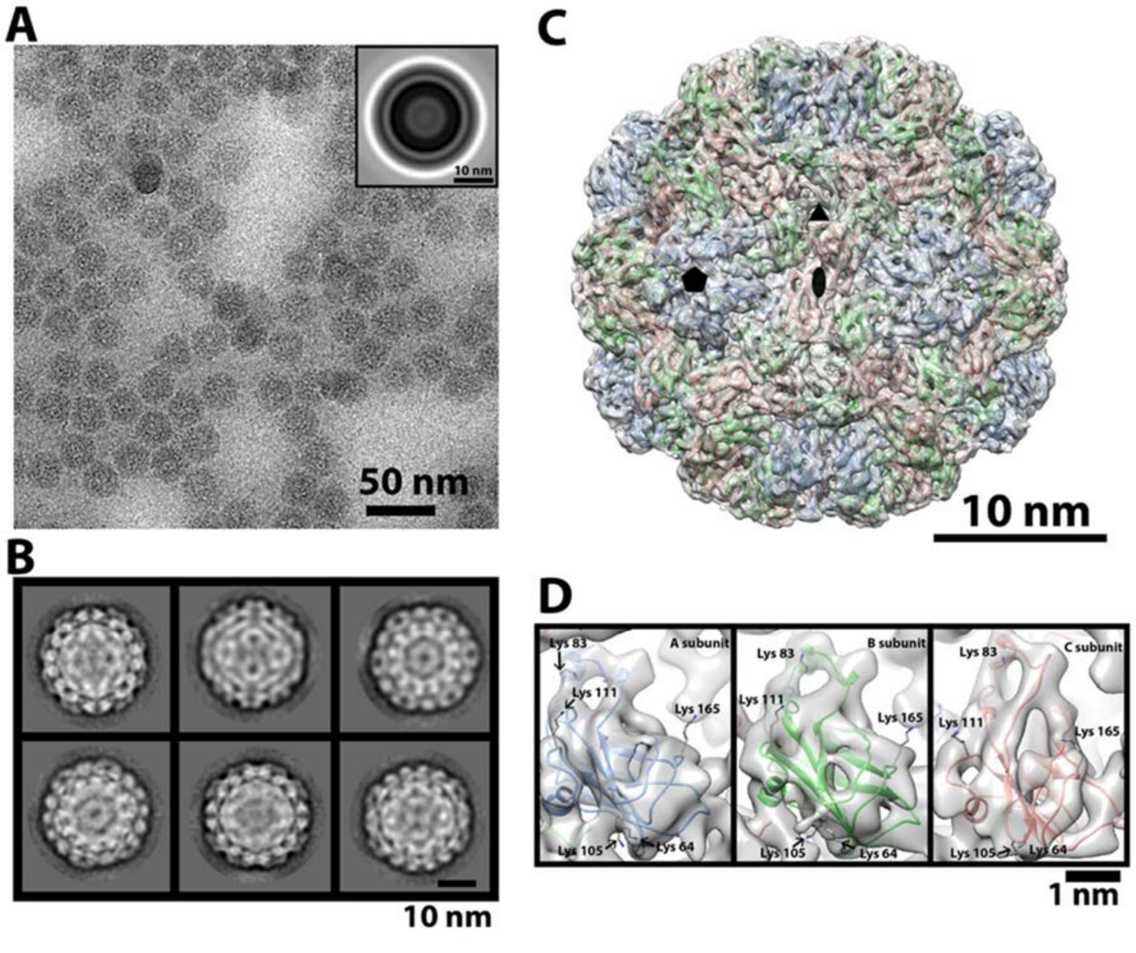


Figure SI4. Cryo-EM analysis of Oregon Green labeled BMV. (A) A representative cryo-EM micrograph of BMV particles vitrified in a thin layer of ice. Inset shows the rotationally aligned averaged image. (B) Selected typical class averages calculated from reference-free 2D classification. (C) The cryo-EM structure of Oregon Green labeled BMV (transparent grey) fitted with the atomic structure of BMV (PDB code 1JS8). (D) Close-up views of each subunits show Lys 64 has become buried within the electron density map.

located at the fivefold axes and 20 hexameric capsomer protrusions located at threefold axes. Docking of the X-ray crystallographic structure (PDB code 1JS9) into the cryo-EM density map reveals excellent agreement (Fig SI4C). Out of five possible locations on the BMV capsid protein that may interact with Oregon Green: Lys 64, Lys 83, Lys 105, Lys 111, and Lys 165. Lys 64 was found to be mostly buried inside the cryo-EM density (FigSI4D). Other Lys positions are either partially exposed or fully exposed.

Since at the current resolution in the Cryo-EM reconstruction no extra density could be attributed to Oregon Green molecule, we surmise the dye must be very close to the BMV surface. This is supported by the dye-conjugated BMV particles being more stable to physical

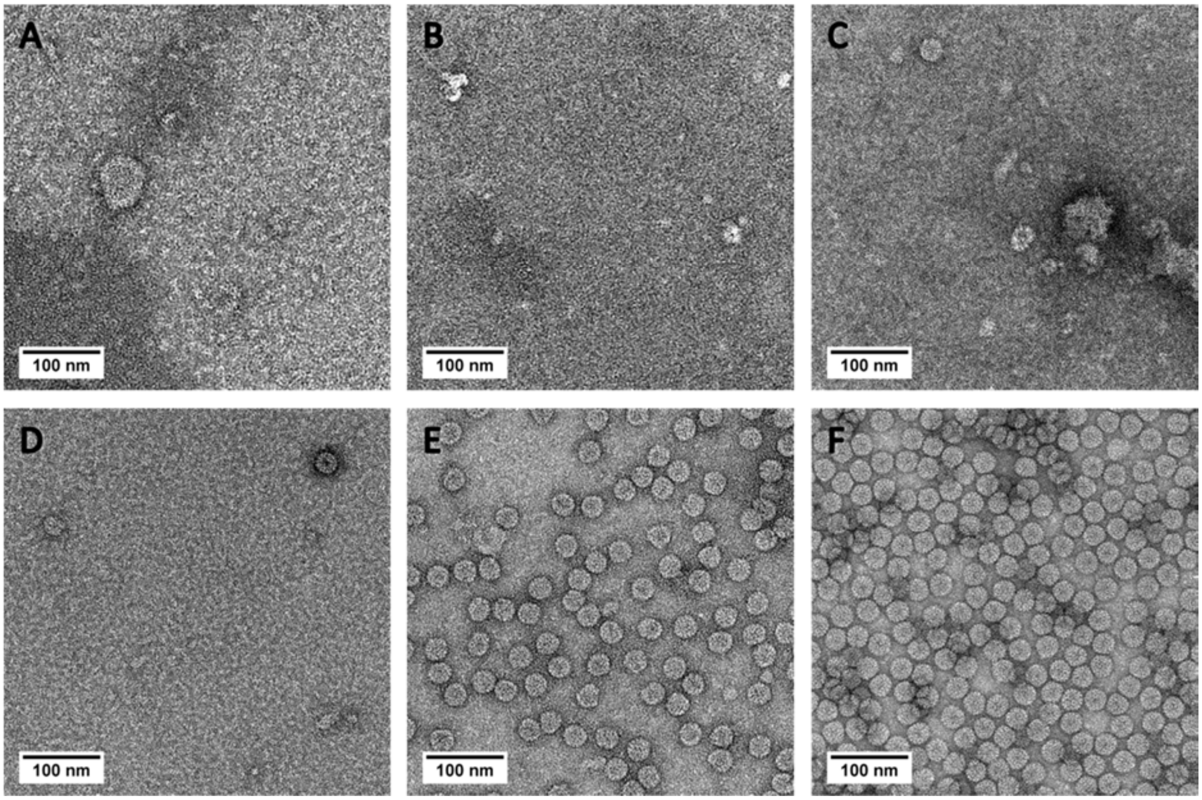


Figure SI5. Stability test. TEM images of samples after overnight dialysis in disassembly buffer: A) wtBMV, B) BOG74 , C) BOG 196, D) BOG 224, E) BOG 268 and F) BOG 288 after drying-reconstitution cycle.

and chemical manipulations with respect to wtBMV, which suggests that the chromophore interacts strongly with the capsid, stabilizing it. Specifically, when dialyzed in disassembly buffer conditions for 24 hours, wtBMV is completely disassembled (Fig. SI5A) but dye-conjugated BMV with dye ratio above 200 has the same morphology as in virus-storage buffer (Fig. SI5D-E). Additionally, the <N>=288 sample was completely dried under vacuum overnight and reconstituted with SAMA buffer. Again, the <N> = 288 virus particles retained their native morphology and optical properties (by FLIM).

**Fluorescence Life-Time Imaging Considerations**

FLIM images are presented in Figure SI6. Non-monotonic changes of photon counts (grey scale) and lifetime (color scale) as function of the average number of dyes per virus particle are visible. The scatter plots presented in the main text were obtained by integrating the photon counts from single virus areas and measuring the mean of photon arrival times for at least 200 single virus particles, and from at least 5 images obtained from different regions in the sample.

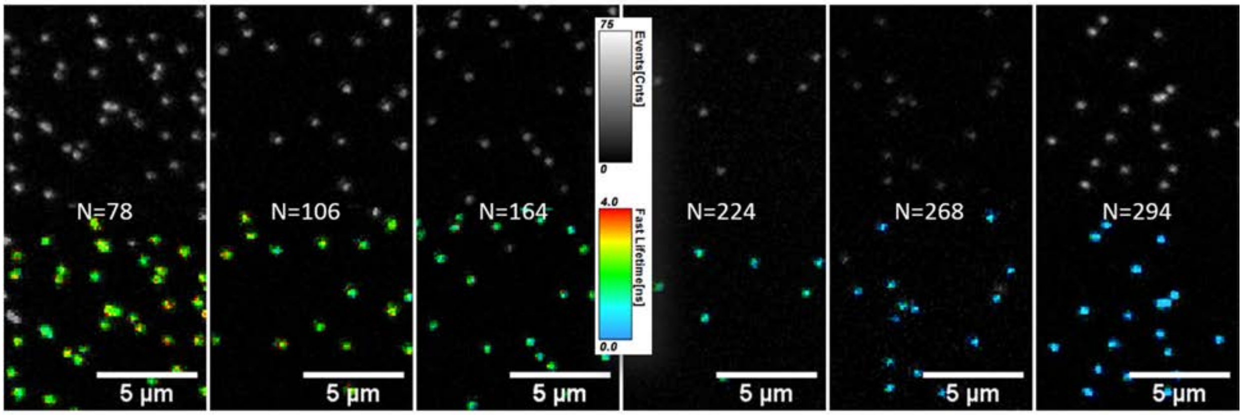


Figure SI6. FLIM images of single particles: photon counts (top row) decreases until N>200 and mean of photon arrival times (bottom row) decreasing from 3.5 ns to 0.5 ns.

We used the mean photon arrival time per pixel as a measure of the single particle lifetime instead of a histogram fit due to the noise in the individual histograms of arrival times at low counts per pixel. In support for this approach giving a fair representation of the lifetime, we integrated the arrival times over all pixels associated with virus particles and used the ensemble histogram for exponential fitting to find the overall sample lifetime. The value thus obtained matched well the averaged mean photon arrival time per pixel.

It is important to note here that the fluorescence life-time microscopy setup is based on the time correlated single photon counting (TCSPC) scheme. While this scheme clearly indicates that the emitted number of photons depends non-linearly on <N>, for quantitative studies TCSPC has the drawback that it relies on the assumption of uncorrelated photon emission statistics, more specifically, on the assumption of one or less photons per pulse. Thus, after the excitation pulse, detection of arrival of the first emitted photon triggers the readout and one event is recorded in the histogram at the arrival time. The TCSPC card is not able to count for a period known as “dead-time” after this event, which in our case is 90 ns. For correlated photons, counts and lifetimes may appear skewed when the TCSPC scheme is used. Work is underway to implement a second-order photon correlation setup, which will be able to provide the true photon correlation statistics.

It is worth noting that at the maximum laser power employed in our setup, we expect photon emission at each pulse. With this assumption and taking into account losses in FLIM set-up (reflections, detector quantum yield, and electronics dead time) we calculated the maximum measurement limit to be 60 photon counts/pixel. By integration over 9 pixels/particle, to include all photons from a single virus, the maximum counts for particle emitted at every pulse,

is in the range of 300-350 counts/particle (because of bell-shaped point-spread function). This is also the maximum we have obtained for samples with N>200. Therefore, the maximum counts obtained for samples with N>200, supports efficient excitation and subsequent emission at every pulse. This is only possible if we assume collective relaxation is more effective than non-radiative quenching.

Figure SI7 presents lifetime vs normalized photon counts by number of dyes per particle. Note the changes in lifetime and photon counts due to quenching or suppression of quenching in case of samples with N>200 under pulsed illumination (Fig. SI7A). The increase of average photon counts per dye for control samples with linker and in swelling conditions is due to quenching suppression caused by an increase in interchromophore distance. While data

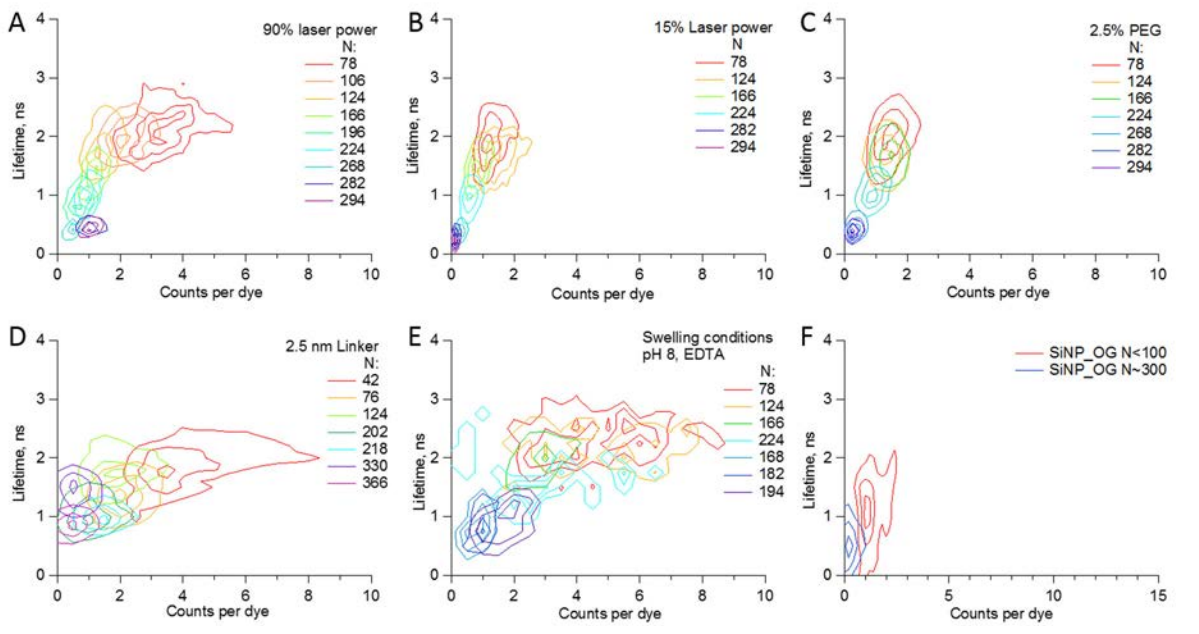


Figure SI7. Contour plots of lifetime vs photon counts normalized by dye number. The different colors represent samples with different average number of chromophores per particle (N). A) 90% laser intensity; B) Same as (A), except for the excitation power 6x less than in (A); C) in the presence of 2.5% PEG 6000; D) with flexible linker between surface lysines and chromophores; E) swelling conditions at pH 8 in the presence of 1mM EDTA, F) Silica nanoparticles decorated with chromophores. Contours correspond to 75%, 60% and 10% of overall population.

shows increased heterogeneity, the overall trend in all control experiments (Fig. SI7B-F) confirms concentration quenching. Based on measured photon counts, one can estimate the degree of fluorescence recovery from quenching to approximately 35%. This value is less than that observed for ensemble measurements (>60%, Fig 5 in main text). The difference may be the result of surface effects since the particles are adsorbed on a glass substrate in this case.

The enhancement factor per dye (Fig SI8) can be defined by:

$$E.F. = \frac{I(N) / \langle I(N_{min}) \rangle}{N \times I_{ss}(N) / I_{ss}(N_{min})} \qquad (1)$$

where $I(N)$ is the photon counts per particle with N chromophores, $N_{min}$ is the minimum N, $I_{ss}(N)$ is photon counts at steady state conditions.

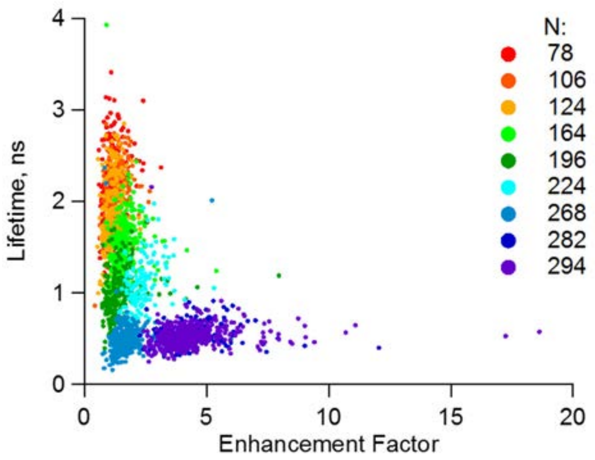


Figure SI8. Scatter plots of lifetime vs enhancement factor per VLP (eq.1). Each dot represent single virus particle. The different colors represent samples with different average number of chromophores per particle (N).

## Control Sample with Flexible Linker

The flexible linker was added between chromophore and virus surface by first reacting the lysines with hetero-bifunctional SMCC (succinimidyl 4-(N-maleimidomethyl)cyclohexane-1-carboxylate, ~8 Å long) and then, adding thiol-TEG-$NH_2$ (~17 Å long), followed by conjugation of OG-488 dye (Fig. SI9A). In this case, it should be noted that some of the dyes were attached to the surface exposed lysines, adding to the heterogeneity of the system and further disrupting symmetry (Fig. SI9C).

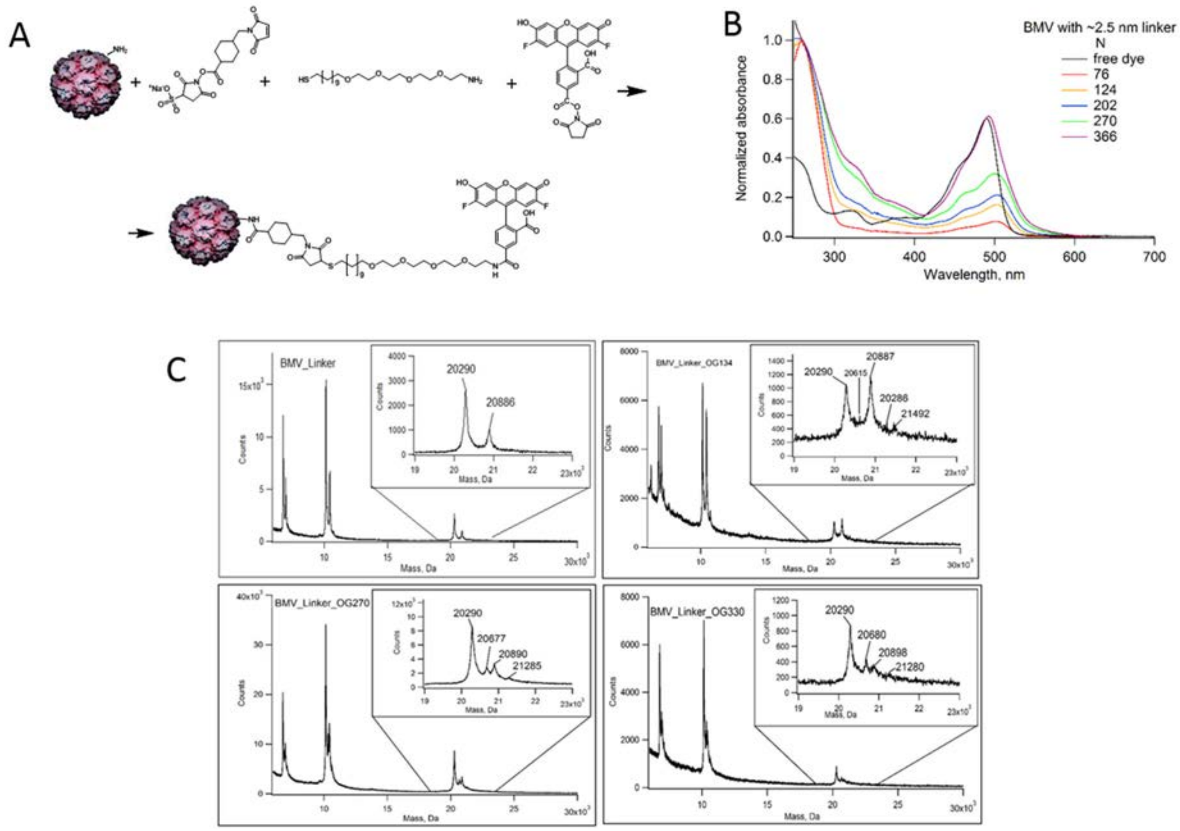


Figure SI9. A) Scheme of bioconjugation through a linker, B) Uv-Vis absorption spectra and C) MALDI-TOF spectra for BMV with flexible linker and samples with dye attached through linker for different N.

## Silica Nanoparticles Control

To investigate the role of the virus template, we performed additional control experiment with a spherical smooth dielectric template. We used amine-modified silica nanoparticles which were functionalized with Oregon green chromophore following same protocol as for BMV samples.

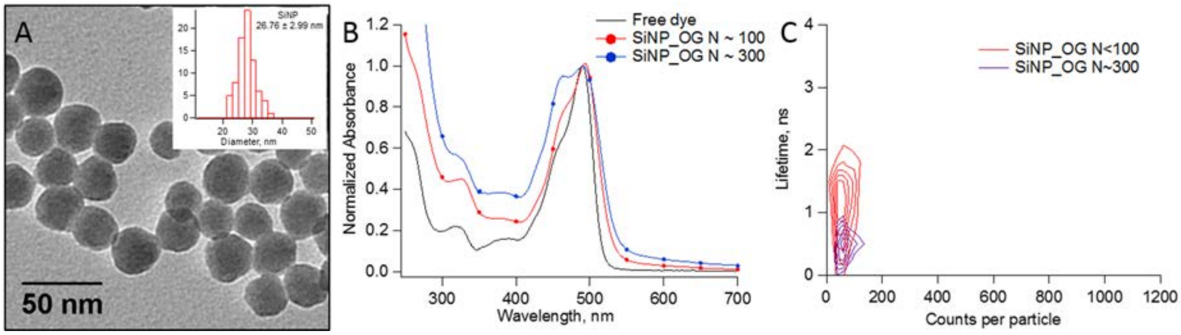


Figure SI10. A) TEM image of SiNP labelled with OG chromophore, inset shows size histogram, B) normalized Uv-Vis absorption spectra and C) Contour plots of lifetime vs fluorescence photon counts collected from hundreds of Silica NP labelled with OG chromophores at 90% laser intensity (same conditions and same scale as figure 3A in main text). Contours surround 75% of the overall population.

The size of silica nanoparticles was chosen close to that of wtBMV (Fig SI10). The Uv-Vis absorption spectra showed significant changes of spectral shape indicative of strong coupling between chromophores even at lower N. FLIM analysis was performed at the same conditions as for BMV_OG samples and emission brightening was not observed (samples with higher N were not detectable in FLIM suggesting strong quenching).

## References


1. Lucas, R.; Larson, S.; McPherson, A., The crystallographic structure of brome mosaic virus. *Journal of Molecular Biology* **2002,** *317* (1), 95-108.
2. Cuillel, M.; Berthetcolominas, C.; Timmins, P. A.; Zulauf, M., Reassembly of Brome Mosaic-virus from dissociated virus - a neutron-scattering study. *Eur. Biophys. J.* **1987,** *15* (3), 169-176.
3. Pfeiffer, F.; Herzog, M.; Hirth, L., RNA viruses - Stabilization of brome mozaic virus. *Philosophical Transactions of the Royal Society of London. B, Biological Sciences* **1976,** *276* (943), 99.
4. Sun, J.; DuFort, C.; Daniel, M.-C.; Murali, A.; Chen, C.; Gopinath, K.; Stein, B.; De, M.; Rotello, V. M.; Holzenburg, A.; Kao, C. C.; Dragnea, B., Core-controlled polymorphism in virus-like particles. *PNAS* **2007,** *104* (4), 1354-1359.
5. Huang, X.; Bronstein, L. M.; Retrum, J.; DuFort, C.; Tsvetkova, I.; Aniagyei, S.; Stein, B.; Stucky, G.; McKenna, B.; Remmes, N.; Baxter, D.; Kao, C. C.; Dragnea, B., Self-assembled virus-like particles with magnetic cores. *Nano Lett.* **2007,** *7* (8), 2407-2416.
6. Dixit, S. K.; Goicochea, N. L.; Daniel, M.-C.; Murali, A.; Bronstein, L.; De, M.; Stein, B.; Rotello, V. M.; Kao, C. C.; Dragnea, B., Quantum dot encapsulation in viral capsids. *Nano Lett.* **2006,** *6* (9), 1993-1999.
7. Yildiz, I.; Tsvetkova, I.; Wen, A. M.; Shukla, S.; Masarapu, M. H.; Dragnea, B.; Steinmetz, N. F., Engineering of Brome mosaic virus for biomedical applications. *Rsc Adv* **2012,** *2* (9), 3670-3677.
8. Running, W. E.; Ni, P.; Kao, C. C.; Reilly, J. P., Chemical reactivity of brome mosaic virus capsid protein. *Journal of molecular biology* **2012,** *423* (1), 79-95.
9. *The Molecular Probes Handbook : a guide to fluorescent probes and labeling technologies.* 11th Edition ed.; Life Technologies: 2010.
